# Supplementary material for: Emergent c-axis magnetic helix in manganite-nickelate superlattices
Source: arXiv:1806.04775 ancillary file (2018-06-12)
Supplement: Supplementary file 1 [file supplemental.pdf]

# Supplemental Material for: Emergent *c*-axis magnetic helix in manganite-nickelate superlattices

G. Fabbris,\* N. Jaouen, D. Meyers, J. Feng, J. D. Hoffman, R. Sutarto, S. G. Chiuabăian, A. Bhattacharya, and M. P. M. Dean<sup>†</sup>  
(Dated: June 12, 2018)

This document provides supporting evidence for the main manuscript. Section I provides x-ray reflectivity and surface x-ray diffraction measurements that demonstrate the  $(\text{La}_{2/3}\text{Sr}_{1/3}\text{MnO}_3)_9/(\text{LaNiO}_3)_3$   $[(\text{LSMO})_9/(\text{LNO})_3]$  high sample quality. In section II, the Ni  $L_3$ -edge RIXS of  $(\text{LSMO})_9/(\text{LNO})_3$  is compared with atomic calculations that assume Ni  $3d^8$  and  $3d^7$  configurations. The x-ray absorption spectroscopy (XAS) and x-ray magnetic circular dichroism (XMCD) data collected at the O  $K$ -, Mn  $L_{3,2}$ - and Ni  $L_2$ -edges are reported in section III.

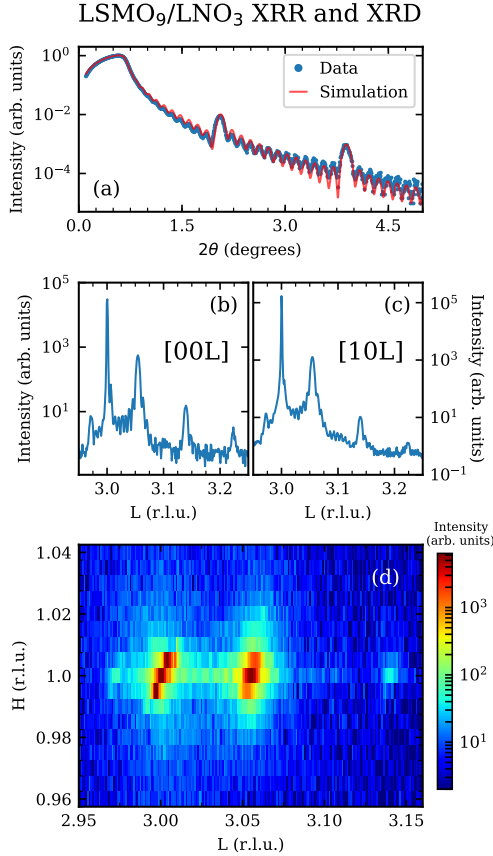

FIG. S1.  $(\text{LSMO})_9/(\text{LNO})_3$  superlattice characterization. (a) XRR data together with a simulation that uses the same structural model as that used in the x-ray resonant magnetic reflectivity reported in the main text. (b)&(c) XRD scans along  $[00L]$  and  $[10L]$  directions, respectively. (d) 2D XRD data around the  $(103)$  reflection. The substrate's reciprocal lattice is used as a reference, thus the sharp peaks at  $(003)$  and  $(103)$  are from  $\text{SrTiO}_3$ .

## I. SAMPLE CHARACTERIZATION

The  $\text{LSMO}_9/\text{LNO}_3$  superlattice studied in the main manuscript was previously investigated in Ref. 1. Nevertheless, we have performed x-ray reflectivity (XRR) and surface x-ray diffraction (XRD) measurements to further confirm the sample quality. Data was collected at room temperature using Cu  $K_\alpha$  radiation from a Brüker D8 Discover equipment. The results are displayed in Fig. S1. Both XRR and XRD measurements show well defined finite thickness fringes and superlattice peaks that are consistent with a good quality sample. Additionally, Figure S1(d) demonstrate that the superlattice  $ab$  plane is strained to the  $\text{SrTiO}_3$  substrate.

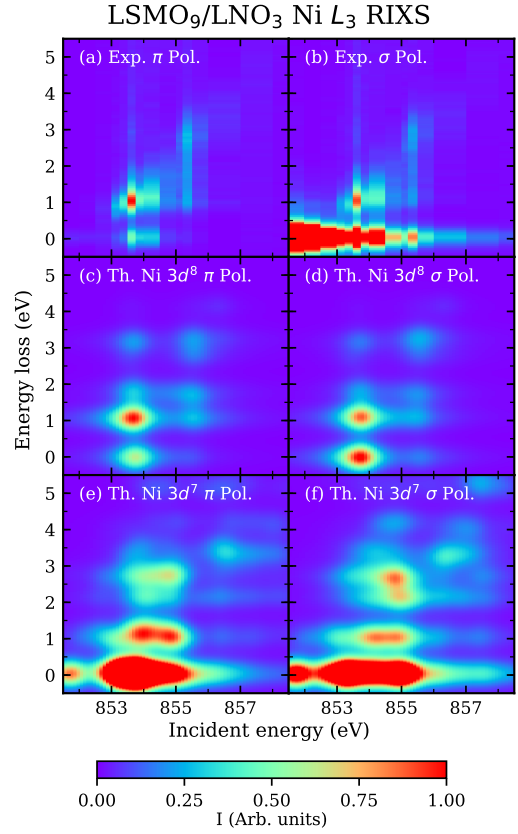

FIG. S2. (a)&(b) display the experimental Ni  $L_3$  RIXS data of  $\text{LSMO}_9/\text{LNO}_3$  collected with  $\pi$  and  $\sigma$  incident x-ray polarization, respectively. Atomic simulations of Ni  $3d^8$  and  $3d^7$  RIXS are shown in panels (c)&(d) and (e)&(f), respectively.

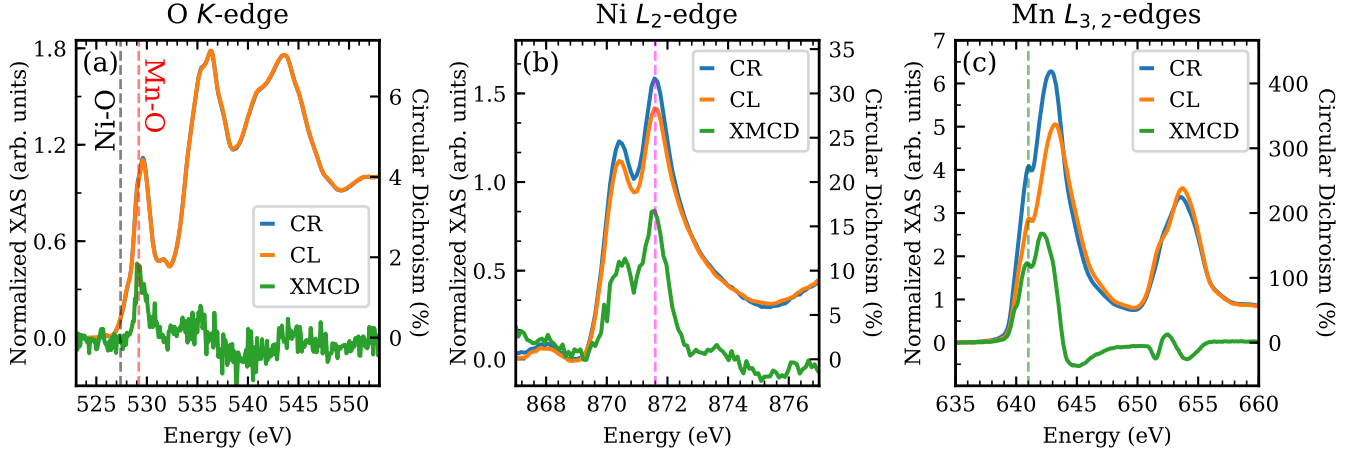

FIG. S3. XAS and XMCD collected at the O  $K$ - (a), Ni  $L_2$ - (b), and Mn  $L_{3,2}$ -edges (c) of the (LSMO)<sub>9</sub>/(LNO)<sub>3</sub> heterostructure. On panel (a), the vertical dashed lines mark the resonant energy of the Ni-O (black) and Mn-O (red) ligand holes. On panels (b)&(c) the dashed lines correspond to the incident x-ray energy used in the data shown on Fig. 3 of the main manuscript.

## II. ATOMIC SIMULATIONS OF NI L-EDGE RIXS

Figure S2 displays the Ni  $L_3$  RIXS data of (LSMO)<sub>9</sub>/(LNO)<sub>3</sub> together with atomic calculations using Ni  $3d^8$  and  $3d^7$  as ground states. These results clearly demonstrate that the (LNO)<sub>3</sub> layers are dominated by Ni  $3d^8$  ions. The experimental result is also markedly distinct from the broad diagonal feature observed in  $RENiO_3$  ( $RE = La$  and  $Nd$ )<sup>2,3</sup>.

## III. X-RAY ABSORPTION SPECTROSCOPY AND X-RAY MAGNETIC CIRCULAR DICHROISM

XAS and XMCD measurements at the O  $K$ -, Mn  $L_{3,2}$ - and Ni  $L_2$ -edges of (LSMO)<sub>9</sub>/(LNO)<sub>3</sub> were performed at the REIXS beamline of the Canadian Light Source. The

data were collected in total electron yield mode and at 20 K. A permanent magnet with a field of 0.6 T was applied and then removed at low temperature, the measurement was thus performed on remanence. The results are displayed in Fig. S3. While the O  $K$ -edge XAS pre-edge is dominated by signal from oxygen ligand holes, the post-edge oscillations are related to both the density of empty states far above the Fermi energy and the photoelectron multiple scattering, thus being less relevant to the current investigation. The XAS and XMCD signal at the Ni  $L_2$ -edge suggests a magnetic Ni<sup>2+</sup> configuration [Fig. S3(b)], in agreement with previous work<sup>1</sup>. The data for the Mn  $L_{3,2}$ -edges are also consistent with previous results<sup>4</sup>. The Ni and Mn XAS and XMCD displayed in Fig. S3 were combined with non-resonant tabulated optical constants<sup>5</sup> to generate the complex index of refraction used in the x-ray resonant magnetic reflectivity (XRMR) simulations. The XRMR fits shown in the main manuscript were performed at the incident x-ray energies marked by the dashed lines in Fig. S3 (b)&(c).

\* gfabbris@anl.gov

† mdean@bnl.gov

<sup>1</sup> Jason D. Hoffman, Brian J. Kirby, Jihwan Kwon, Gilberto Fabbri, D. Meyers, John W. Freeland, Ivar Martin, Olle G. Heinonen, Paul Steadman, Hua Zhou, Christian M. Schlepütz, Mark P. M. Dean, Suzanne G. E. te Velthuis, Jian-Min Zuo, and Anand Bhattacharya, “Oscillatory Non-collinear Magnetism Induced by Interfacial Charge Transfer in Superlattices Composed of Metallic Oxides,” *Physical Review X* **6**, 041038 (2016).

<sup>2</sup> Valentina Bisogni, Sara Catalano, Robert J. Green, Marta Gibert, Raoul Scherwitzl, Yaobo Huang, Vladimir N. Strocov, Pavlo Zubko, Shadi Balandeh, Jean-Marc Triscone, George Sawatzky, and Thorsten Schmitt, “Ground-state

oxygen holes and the metalinsulator transition in the negative charge-transfer rare-earth nickelates,” *Nature Communications* **7**, 13017 (2016).

<sup>3</sup> G. Fabbri, D. Meyers, J. Okamoto, J. Pellicciari, A. S. Disa, Y. Huang, Z. Y. Chen, W. B. Wu, C. T. Chen, S. Ismail-Beigi, C. H. Ahn, F. J. Walker, D. J. Huang, T. Schmitt, and M. P. M. Dean, “Orbital engineering in nickelate heterostructures driven by anisotropic oxygen hybridization rather than orbital energy levels,” *Physical Review Letters* **117**, 147401 (2016).

<sup>4</sup> C. Aruta, G. Ghiringhelli, V. Bisogni, L. Braicovich, N. B. Brookes, A. Tebano, and G. Balestrino, “Orbital occupation, atomic moments, and magnetic ordering at interfaces of manganite thin films,” *Physical Review B* **80**, 014431

(2009).

- <sup>5</sup> C. T. Chantler, “Theoretical Form Factor, Attenuation, and Scattering Tabulation for  $Z = 192$  from  $E = 110$  eV to  $E$

$= 0.41.0$  MeV,” *Journal of Physical and Chemical Reference Data* **24**, 71–643 (1995).
